# Supplementary material for: An Embarrassingly Pragmatic Introduction to Vision-based Autonomous Robots
Source: arXiv:2112.05534 source file (2021-12-14)
Supplement: Supplementary file 1 [file appendix2.tex]

%!TEX root = ../thesis.tex
% ******************************* Thesis Appendix B ********************************

\chapter{Robot and Hardware Setup}
\label{app:robot}

\section{JetBot}

\begin{figure}[!ht]
\includegraphics[trim={0 0 0 0 },clip, width=\textwidth]{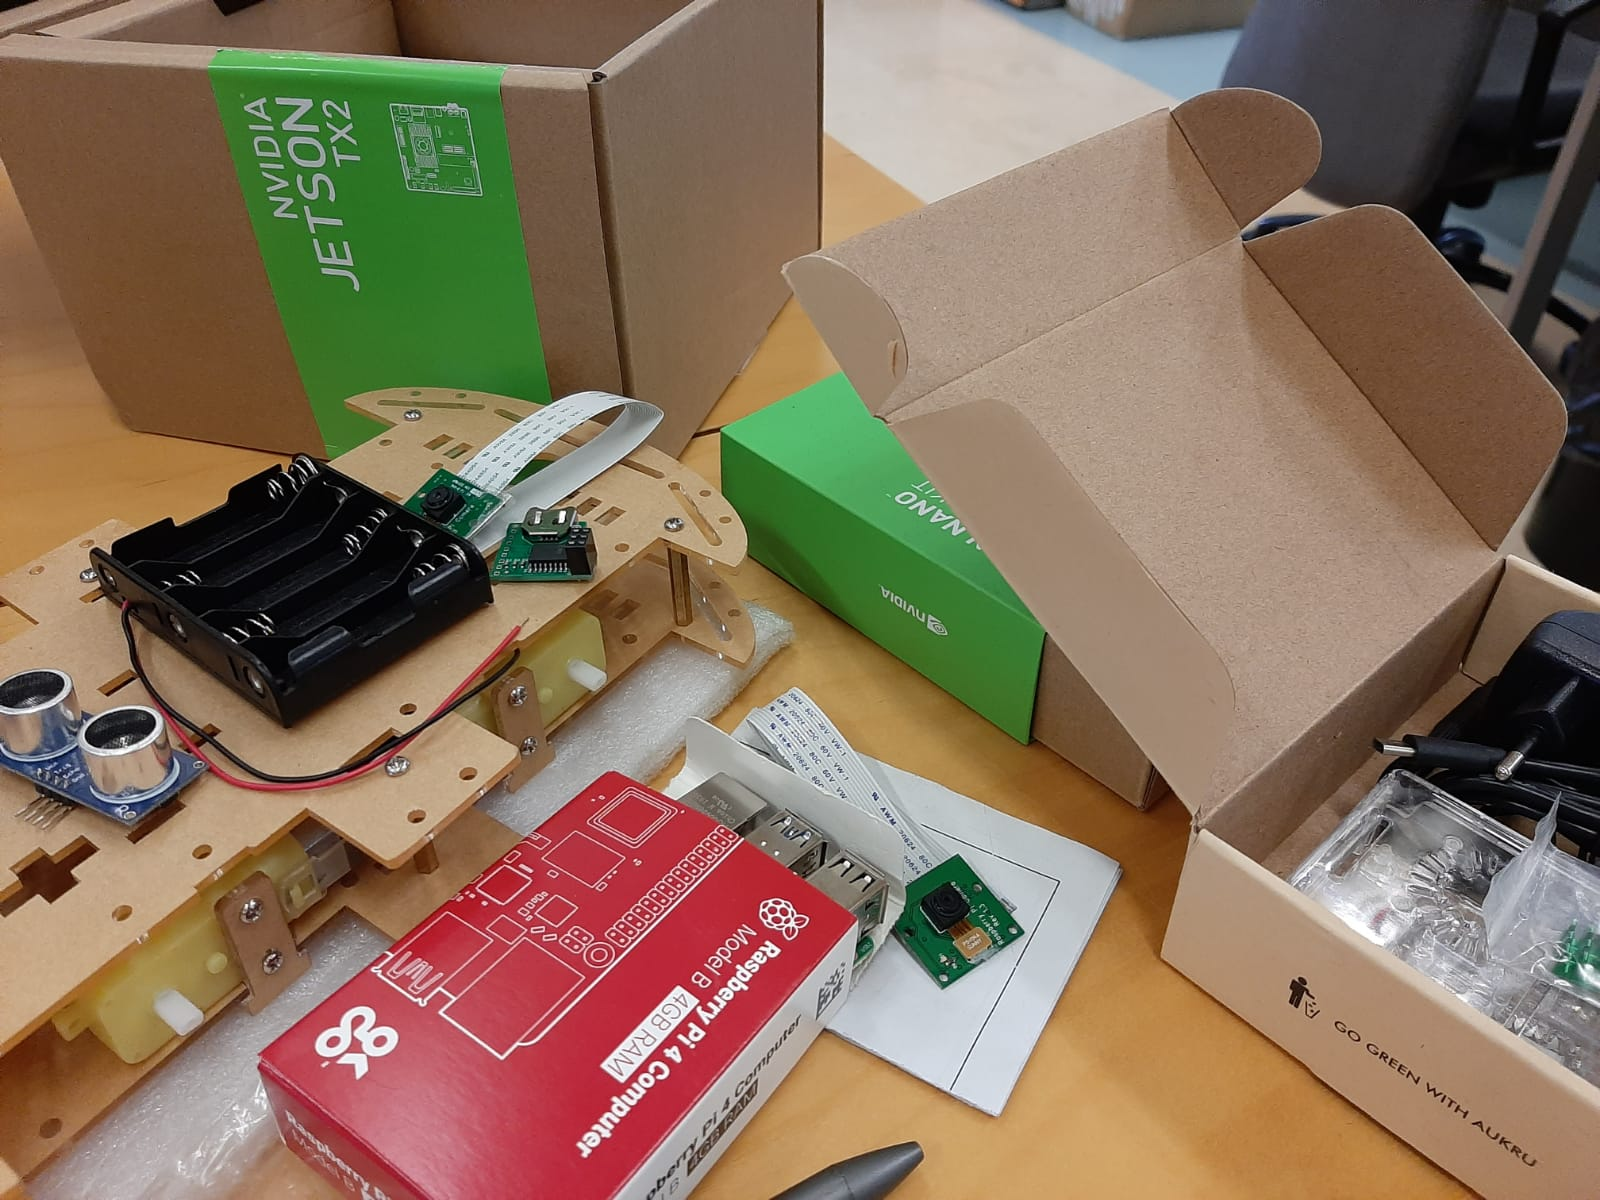}
\centering
\caption[JetBot Unboxing]{JetBot Unboxing}
\label{fig:jetbot-unboxing}
\end{figure}

\begin{figure}[!ht]
\includegraphics[trim={0 0 0 0 },clip, width=0.6\textwidth]{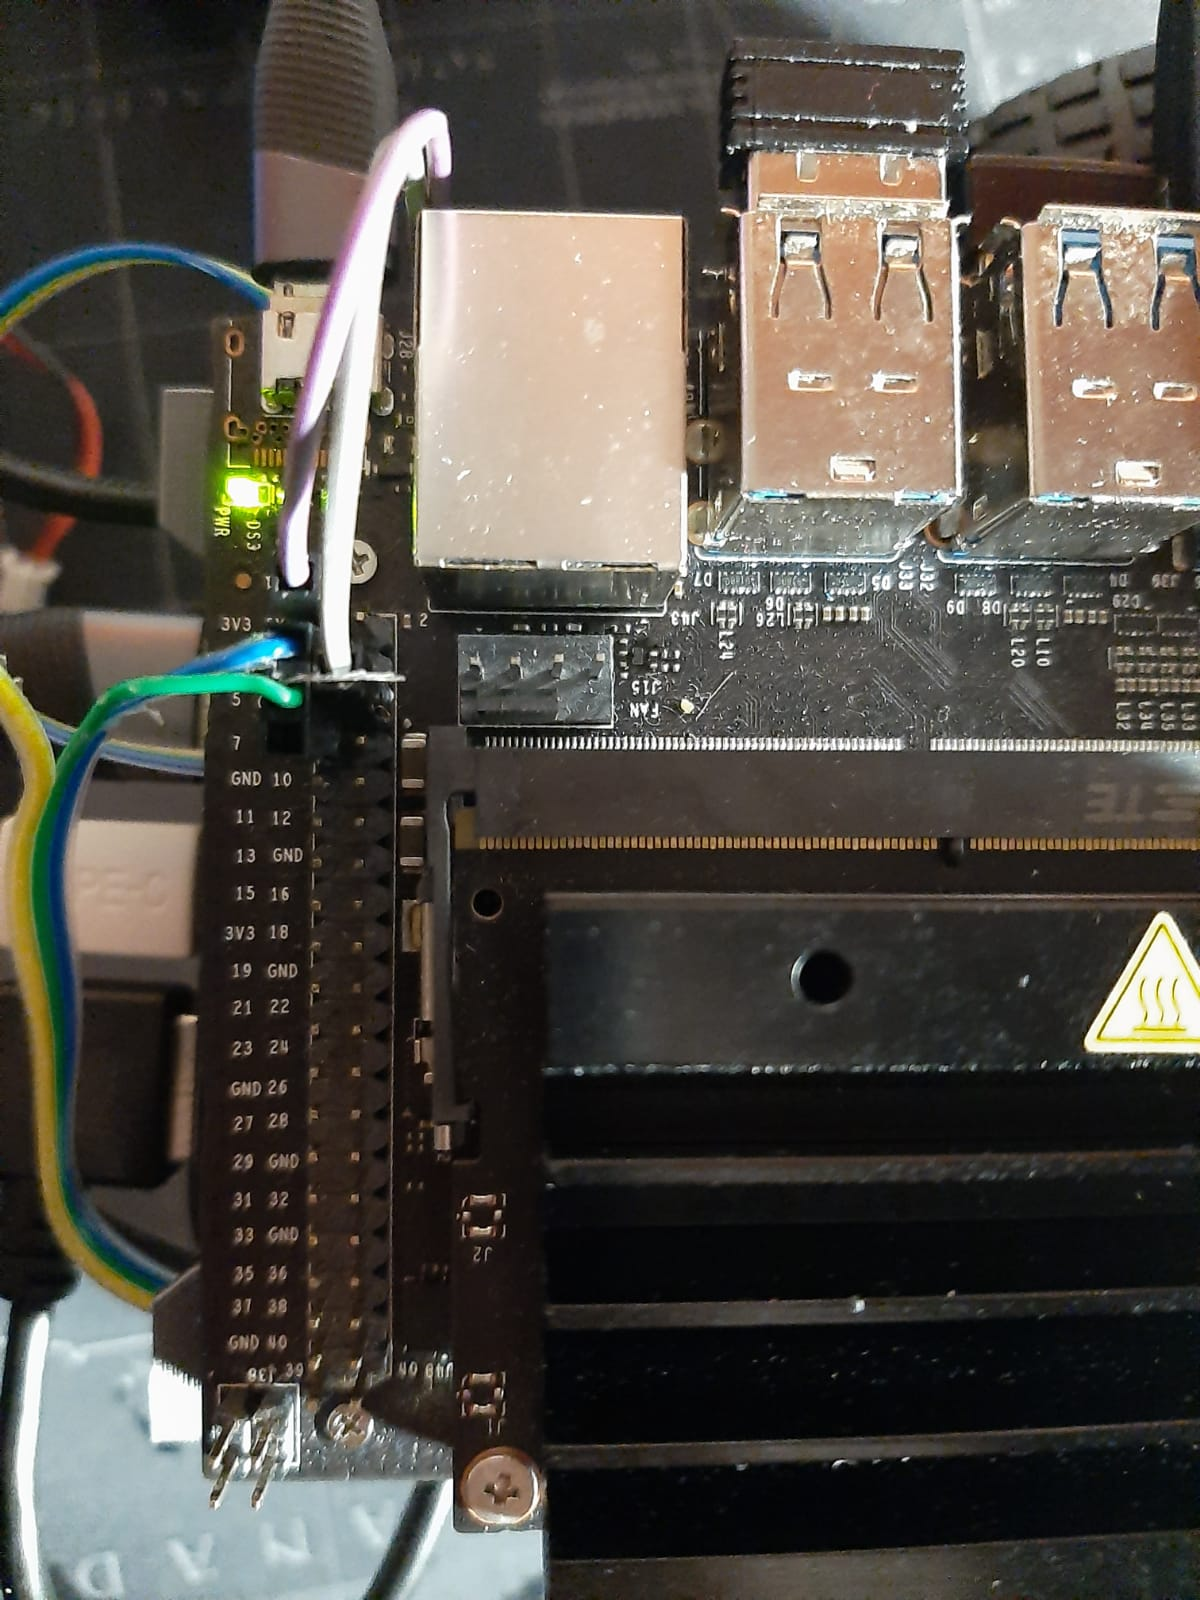}
\centering
\caption[JetBot Motor Connections]{JetBot Motor Connections}
\label{fig:jetbot-connections}
\end{figure}

\begin{figure}[!ht]
\includegraphics[trim={0 0 0 0 },clip, width=0.7\textwidth]{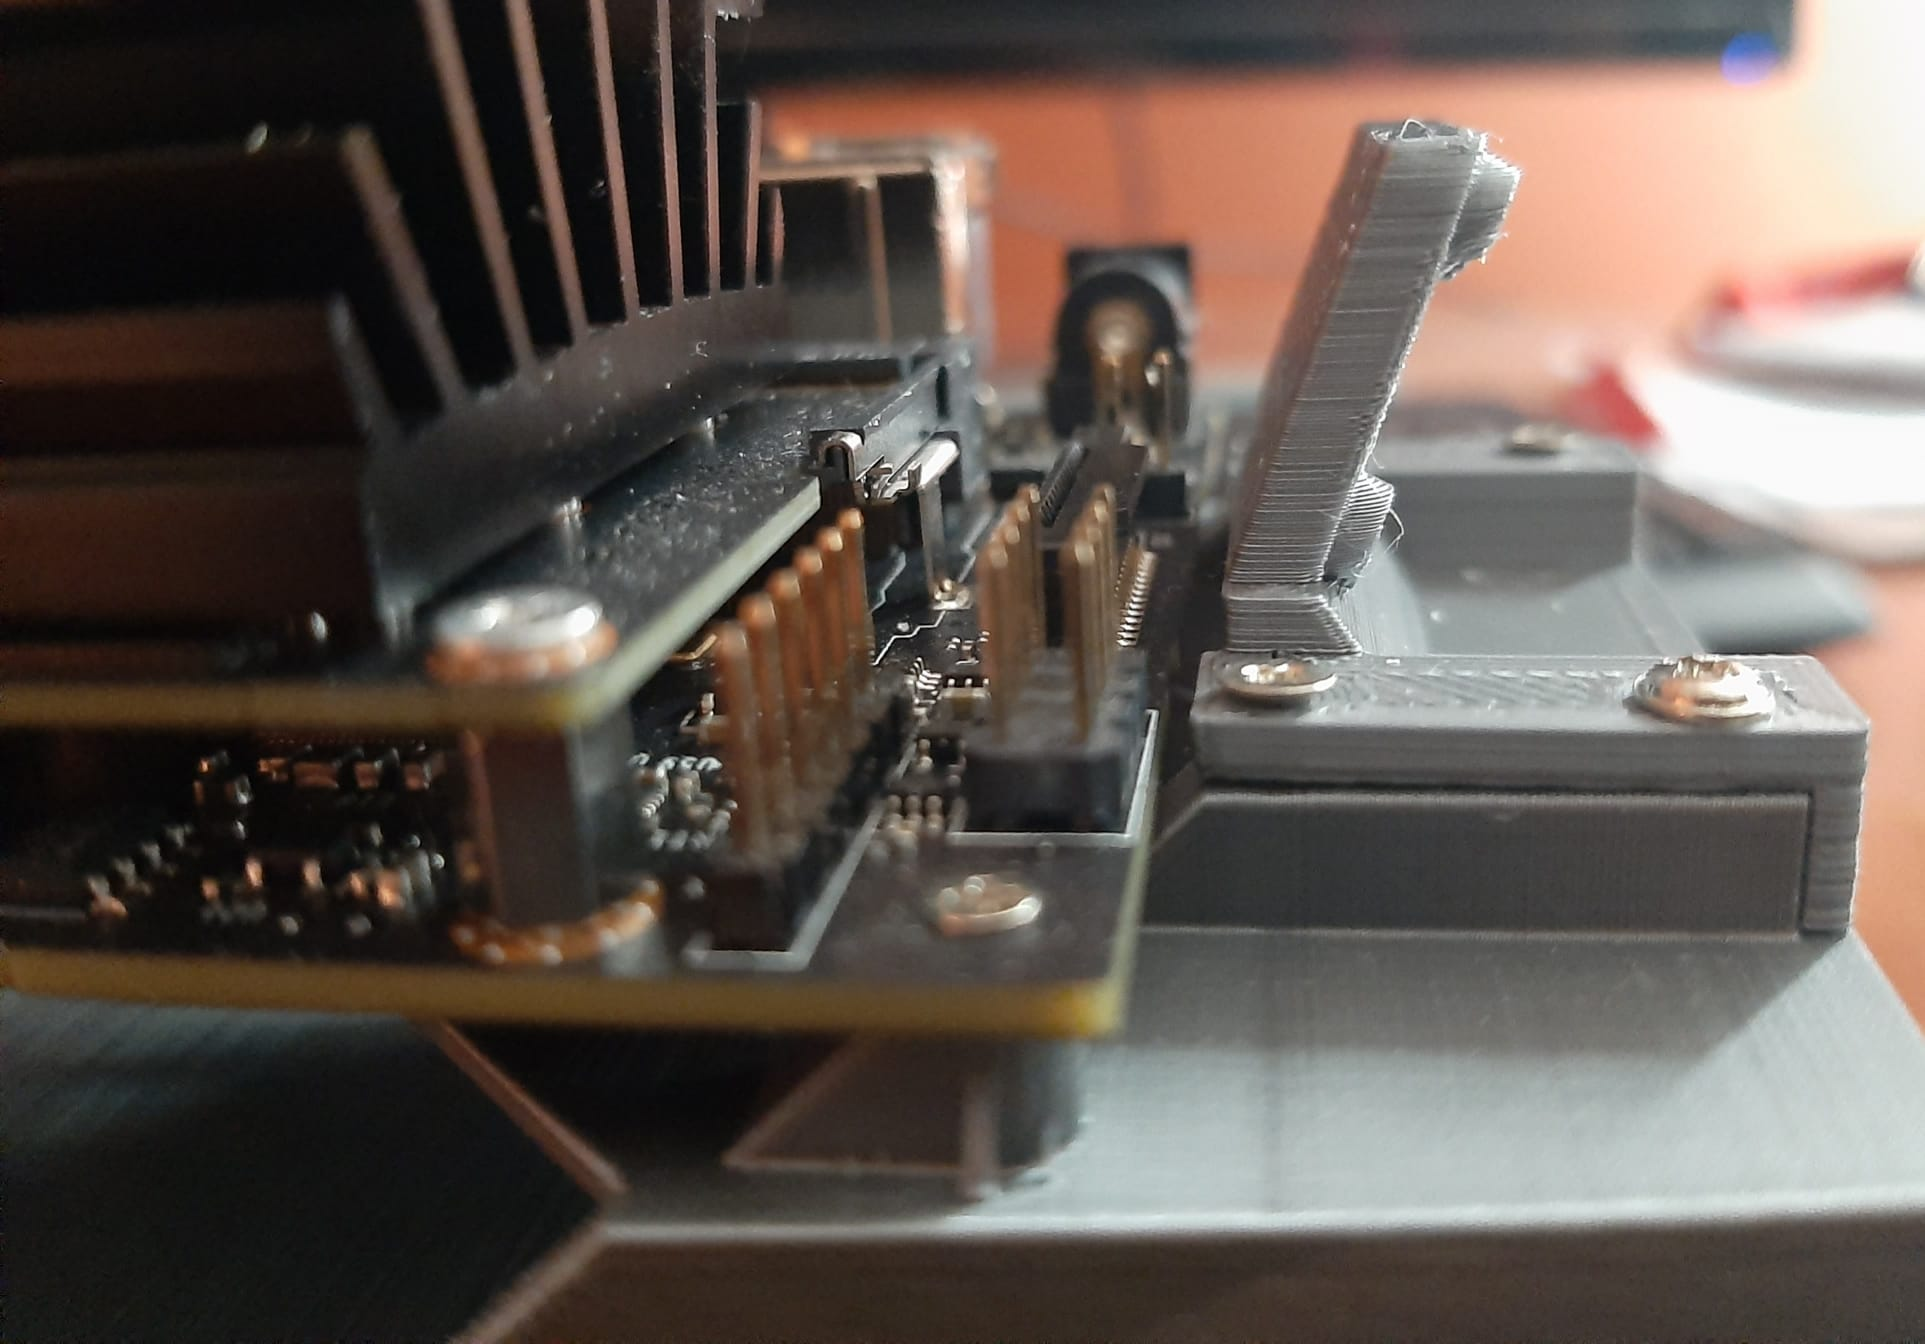}
\centering
\caption[JetBot 3D printed camera support]{JetBot 3D printed camera support}
\label{fig:jetbot-cam}
\end{figure}

\begin{figure}[!ht]
\includegraphics[trim={0 0 0 7cm },clip, width=0.8\textwidth]{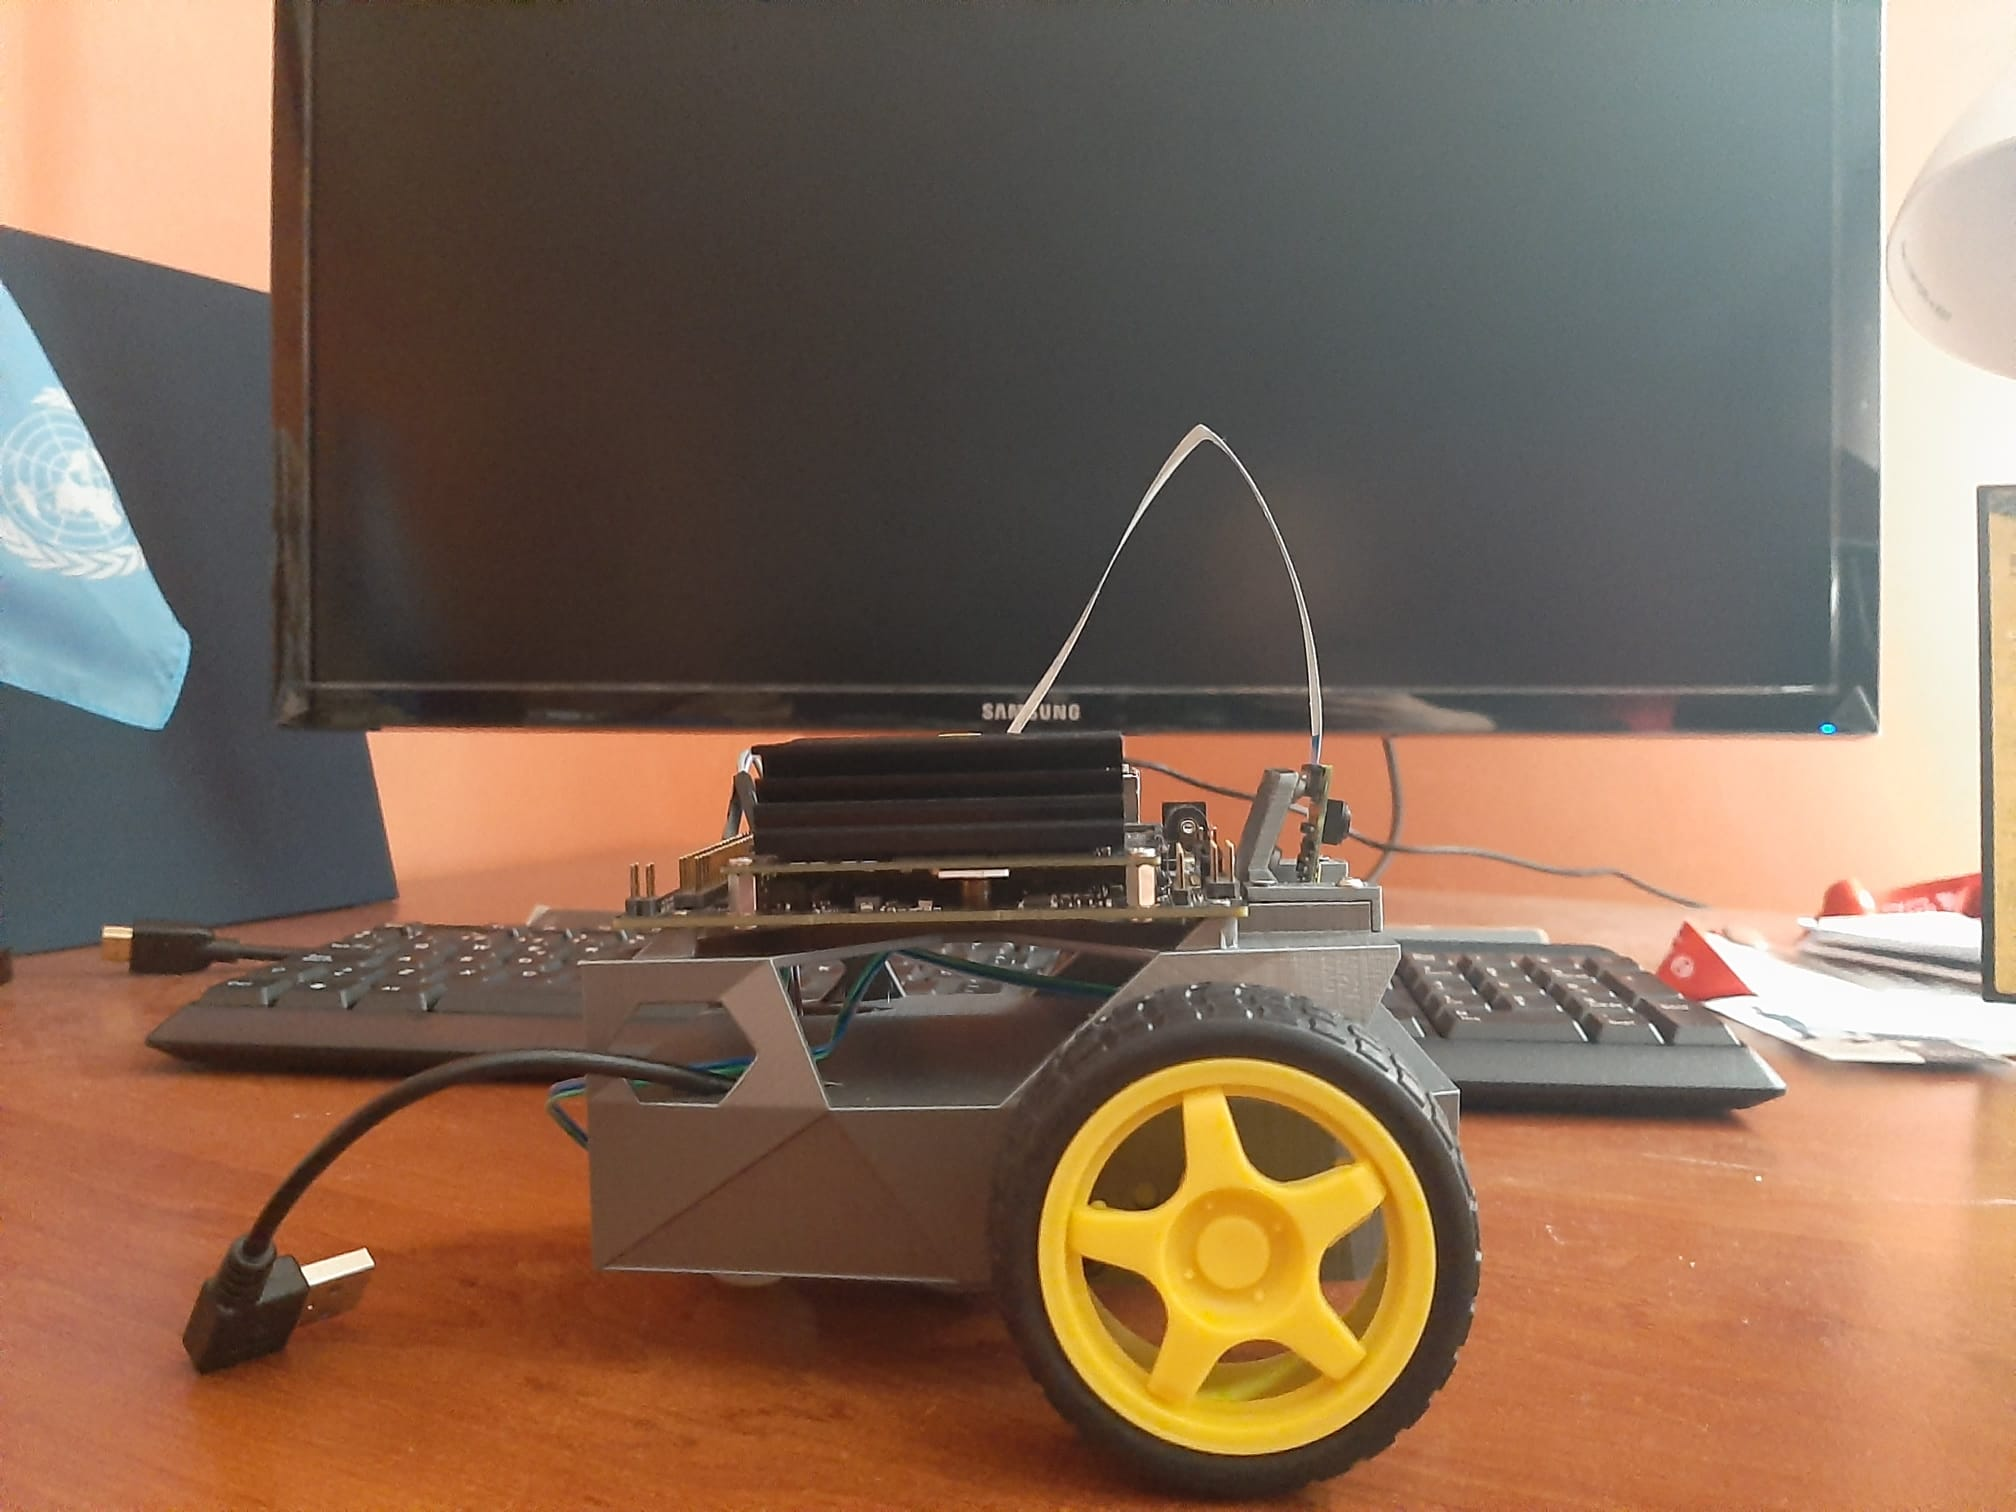}
\centering
\caption[Our JetBot]{Our JetBot}
\label{fig:jetbot}
\end{figure}

\begin{figure}[!ht]
\includegraphics[trim={0 0 0 0 },clip, width=0.8\textwidth]{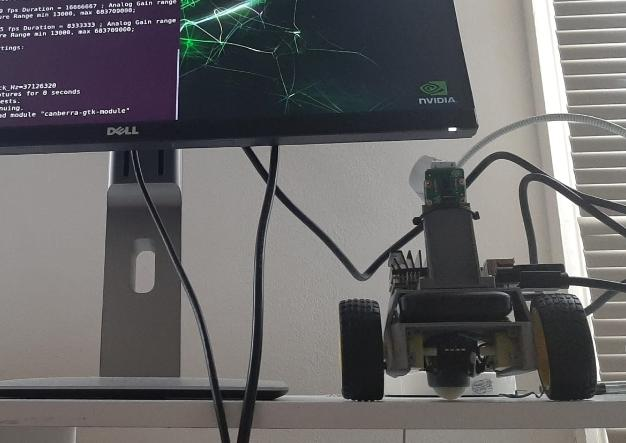}
\centering
\caption[Our JetBot - Front]{Our JetBot - Front}
\label{fig:jetbot-front}
\end{figure}

\clearpage

The JetBot \footnote{\url{https://jetbot.org/master/}} educational robot from NVIDIA was our first try. 
The bill of materials is shown in Table \ref{tab:jetbot-cost}, the total cost of the robot was 200\$. Note that 3D printed parts as the chasis and camera mount, and other generic hardware (skews, usb cable, etc.) are not considered as cost.
We prepare the setup proposed at the official project site (Figure \ref{fig:jetbot-setup}).

To improve efficiency and performance, we install Linux Mint, a lighter Linux distribution than the proposed Ubuntu, and LXDE Desktop Environment, by doing this we save up to 1.5 GB of RAM thanks to the operating system. The complete setup took around 4hrs.

\begin{figure}[!ht]
\includegraphics[trim={0 0 0 0 },clip, width=0.78\textwidth]{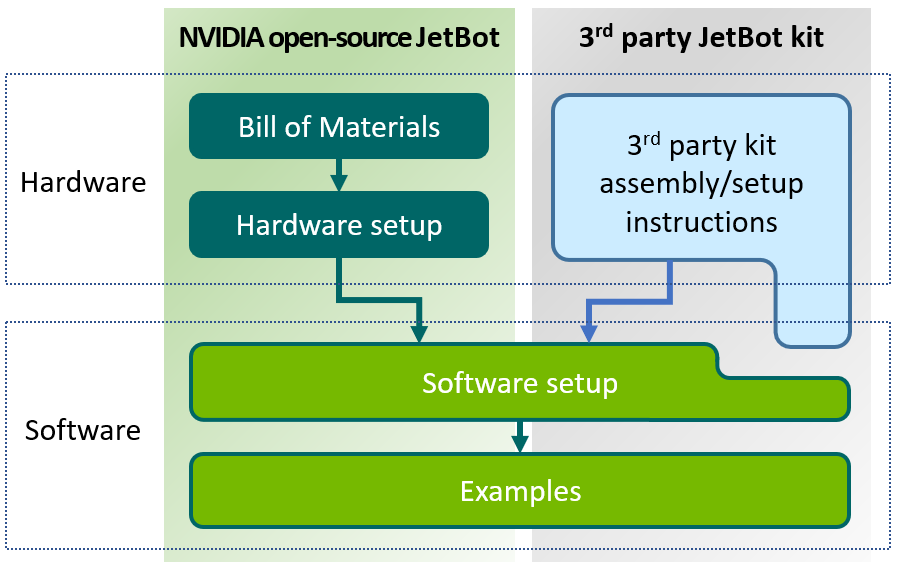}
\centering
\caption[JetBot setup]{JetBot setup. After completing the hardware setup and building up the robot (DIY version), we start the software setup.}
\label{fig:jetbot-setup}
\end{figure}

\begin{table}[]
    \centering
    \caption{JetBot Bill of Materials.}
    \begin{tabular}{l c}
         Part & Cost (\$) \\
         \toprule
         Jetson Nano & 100 \\
         Power supply & 14 \\
         Battery & 16 \\
         Caster ball & 7 \\
         Motor & 6 \\
         Motor Driver & 20 \\
         Micro SD card & 15 \\
         Camera RPi Camera V2  & 25 \\
         \midrule
         Total  & 200 \\
         \bottomrule
    \end{tabular}
    \label{tab:jetbot-cost}
\end{table}

Figures \ref{fig:jetbot-unboxing}, \ref{fig:jetbot-connections}, \ref{fig:jetbot-cam} show the unboxing of the material and building process (3d printed parts, wire connections, etc.). Figures \ref{fig:jetbot}, \ref{fig:jetbot-front} show our final DIY JetBot robot.

\paragraph{NVIDIA Jetson Nano vs Raspberry Pi 4}

The NVIDIA Jetson Nano (2019) and Raspberry Pi 4 (2019) are widely the most used computers for embedded designers, researchers, and DIY makers, delivering the power of modern AI in a compact board. The following table shows the main differences between both computers:

\begin{figure}[!ht]
\includegraphics[trim={0 0 0 0 },clip, width=\textwidth]{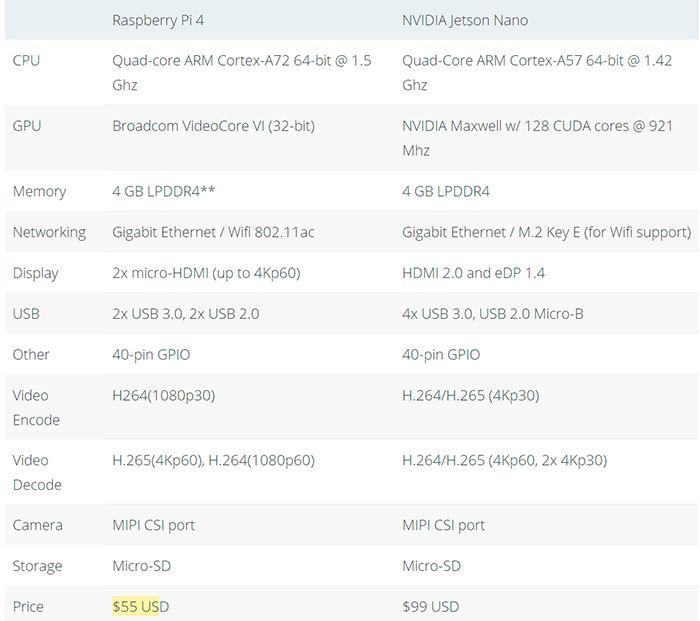}
\centering
\caption[Jetson Nano vs Raspberry Pi 4]{Jetson Nano vs Raspberry Pi 4.}
\label{fig:jetson_vs_rpi}
\end{figure}

As we can see in Figure \ref{fig:jetson_vs_rpi}, the main features of both boards are similar. However, there is an important distinction, the biggest difference and the reason why we chose the Jetson Nano lies in the graphics capabilities and its GPU (28-core Maxwell GPU at 921 MHz) which makes the Jetson Nano more suitable for AI and ML applications.

\paragraph{How to control it remotely?} 

The JetBot project includes initial examples for: Basic Motion, Teleoperation, Collision Avoidance, Road Following and Object Following \footnote{\url{https://jetbot.org/master/examples/basic_motion.html}}.
Using the official software from GitHub \footnote{\url{https://github.com/NVIDIA-AI-IOT/jetbot}} we install all the needed libraries and APIs to control the servo motors and camera. We send JetBot commands and get camera information (image stream) using Python scripts and Jupyter Notebooks.

\begin{figure}[!ht]
\includegraphics[trim={0 0 0 0 },clip, width=0.8\textwidth]{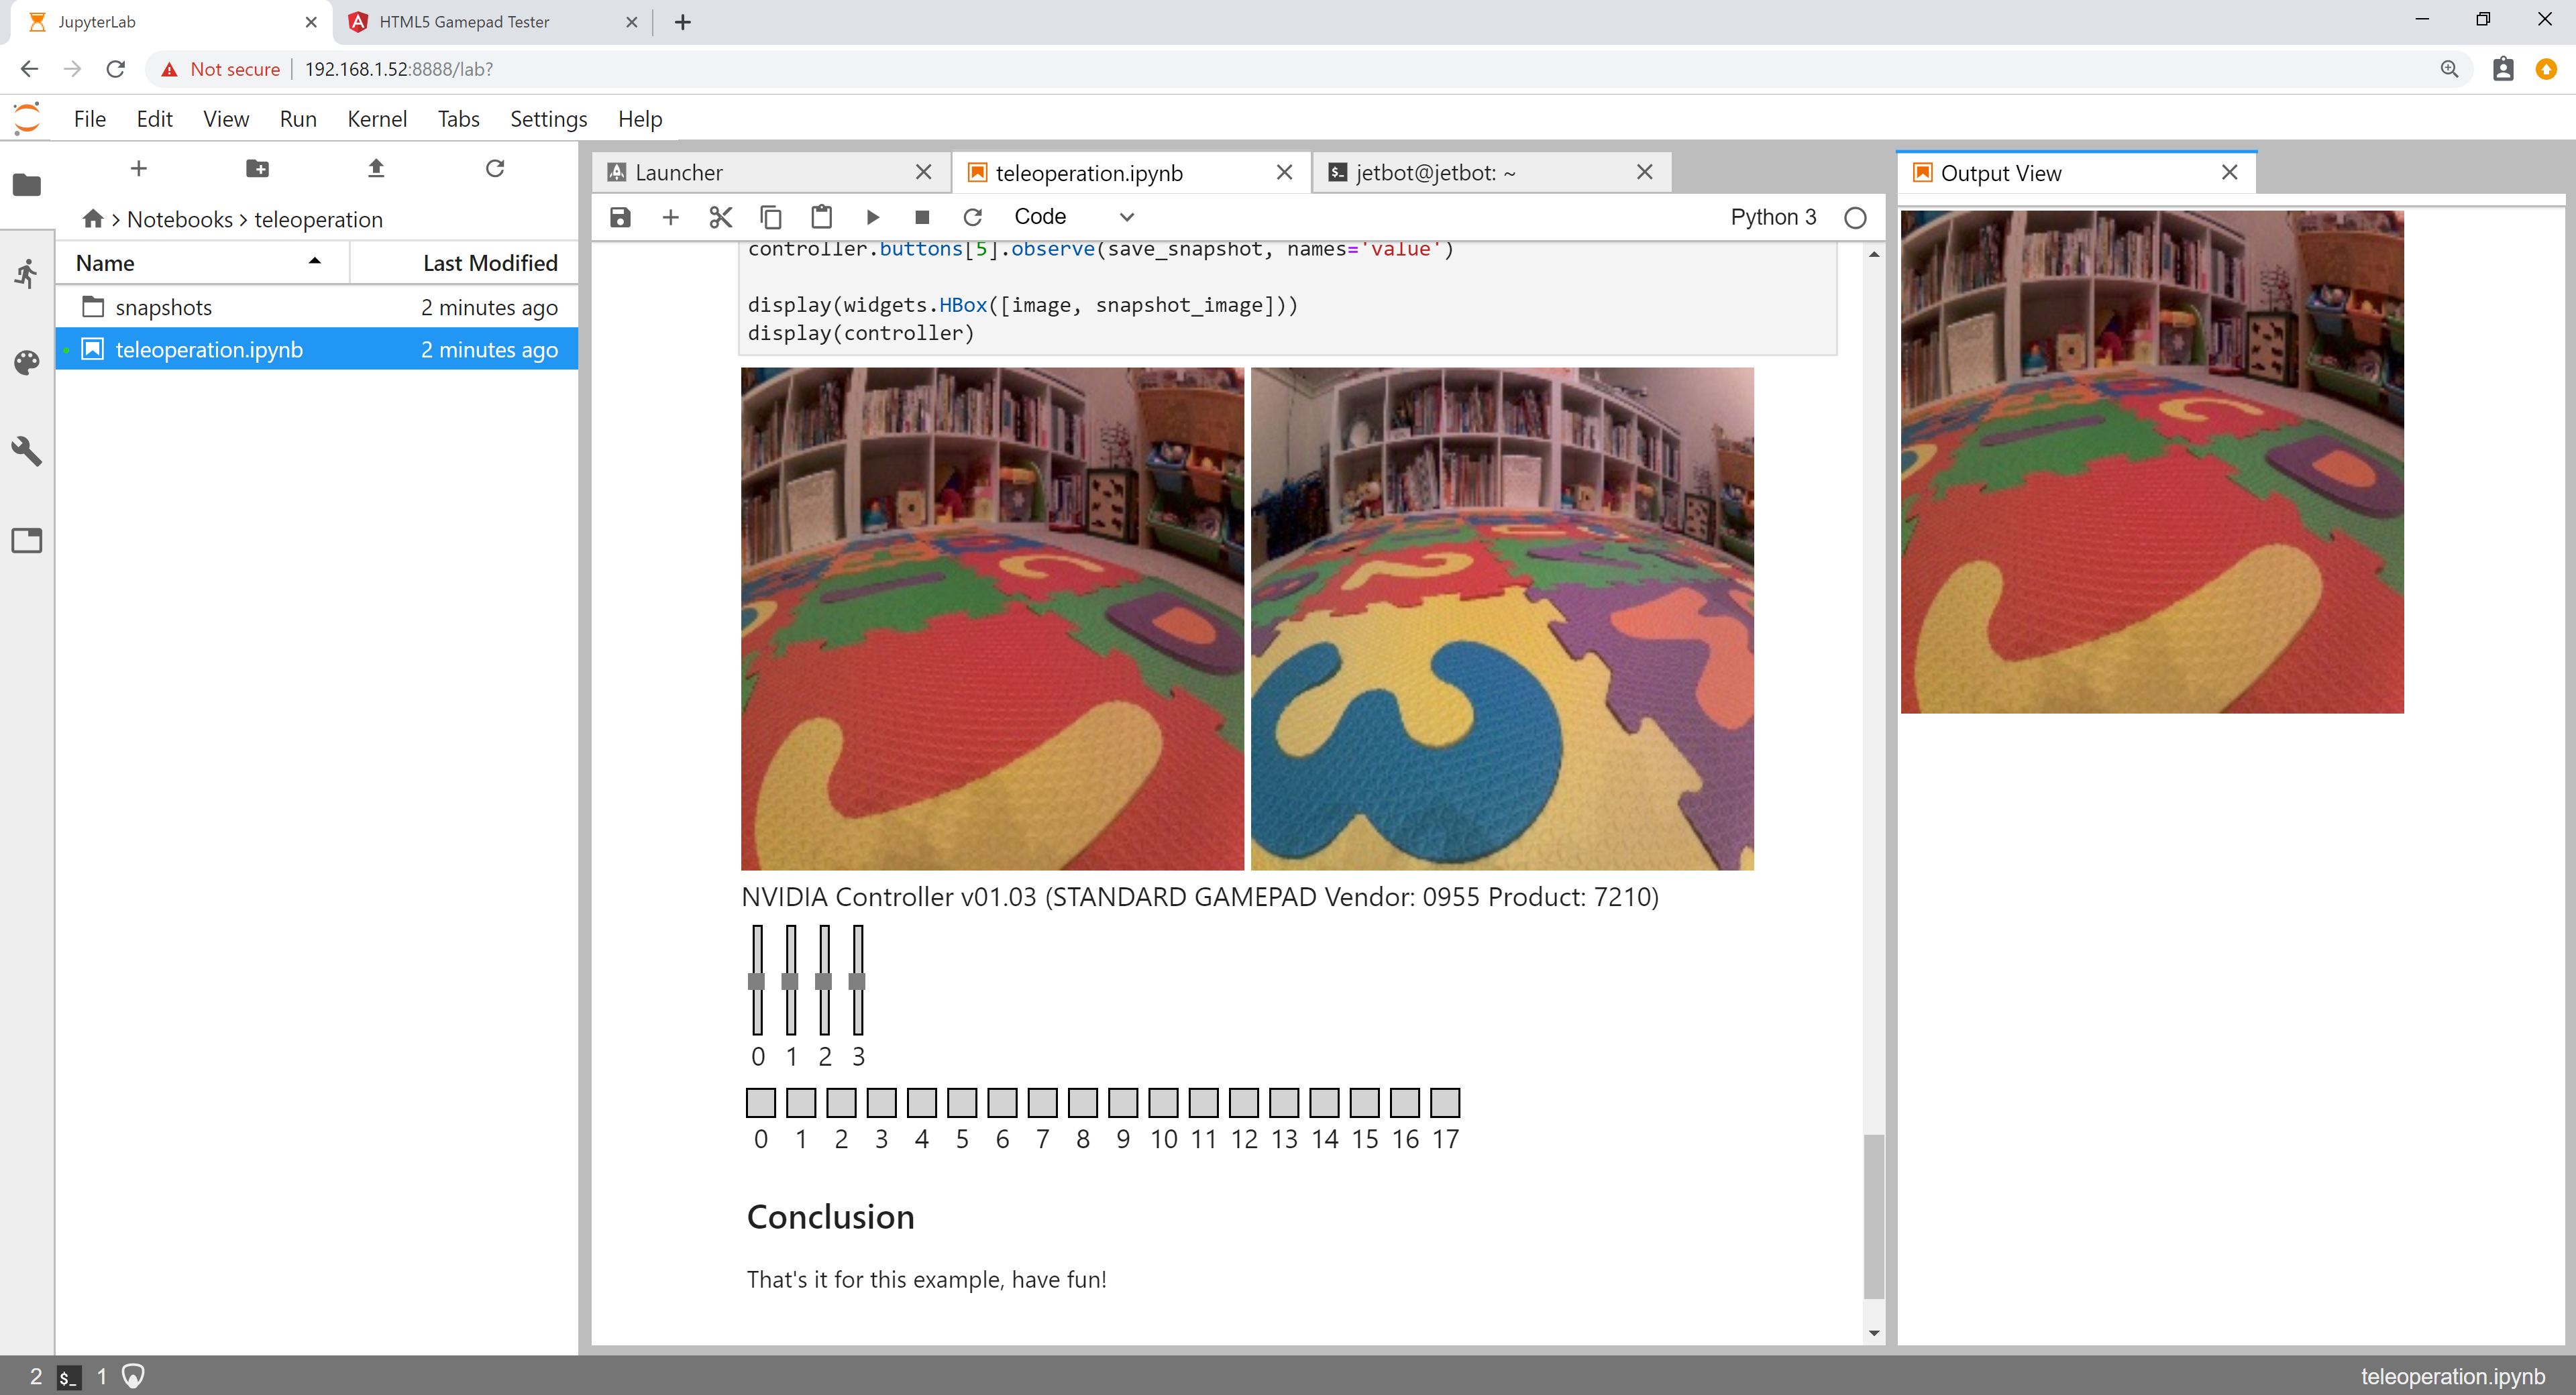}
\centering
\caption[JetBot Teleoperation Example]{JetBot Teleoperation Example from offcial tutorial.}
\label{fig:jetbot-interface}
\end{figure}

\begin{figure}[!ht]
\includegraphics[trim={0 0 0 0 },clip, width=0.8\textwidth]{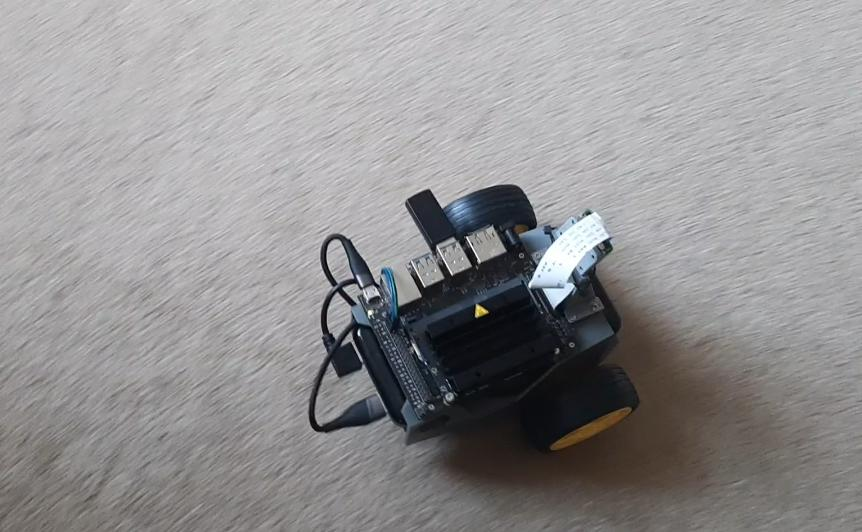}
\centering
\caption[Our JetBot Working]{Our JetBot Working.}
\label{fig:jetbot-working}
\end{figure}

\clearpage
\section{JetRover}

\begin{figure}[!h]
\includegraphics[trim={0 15cm 0 0 },clip, width=0.5\textwidth]{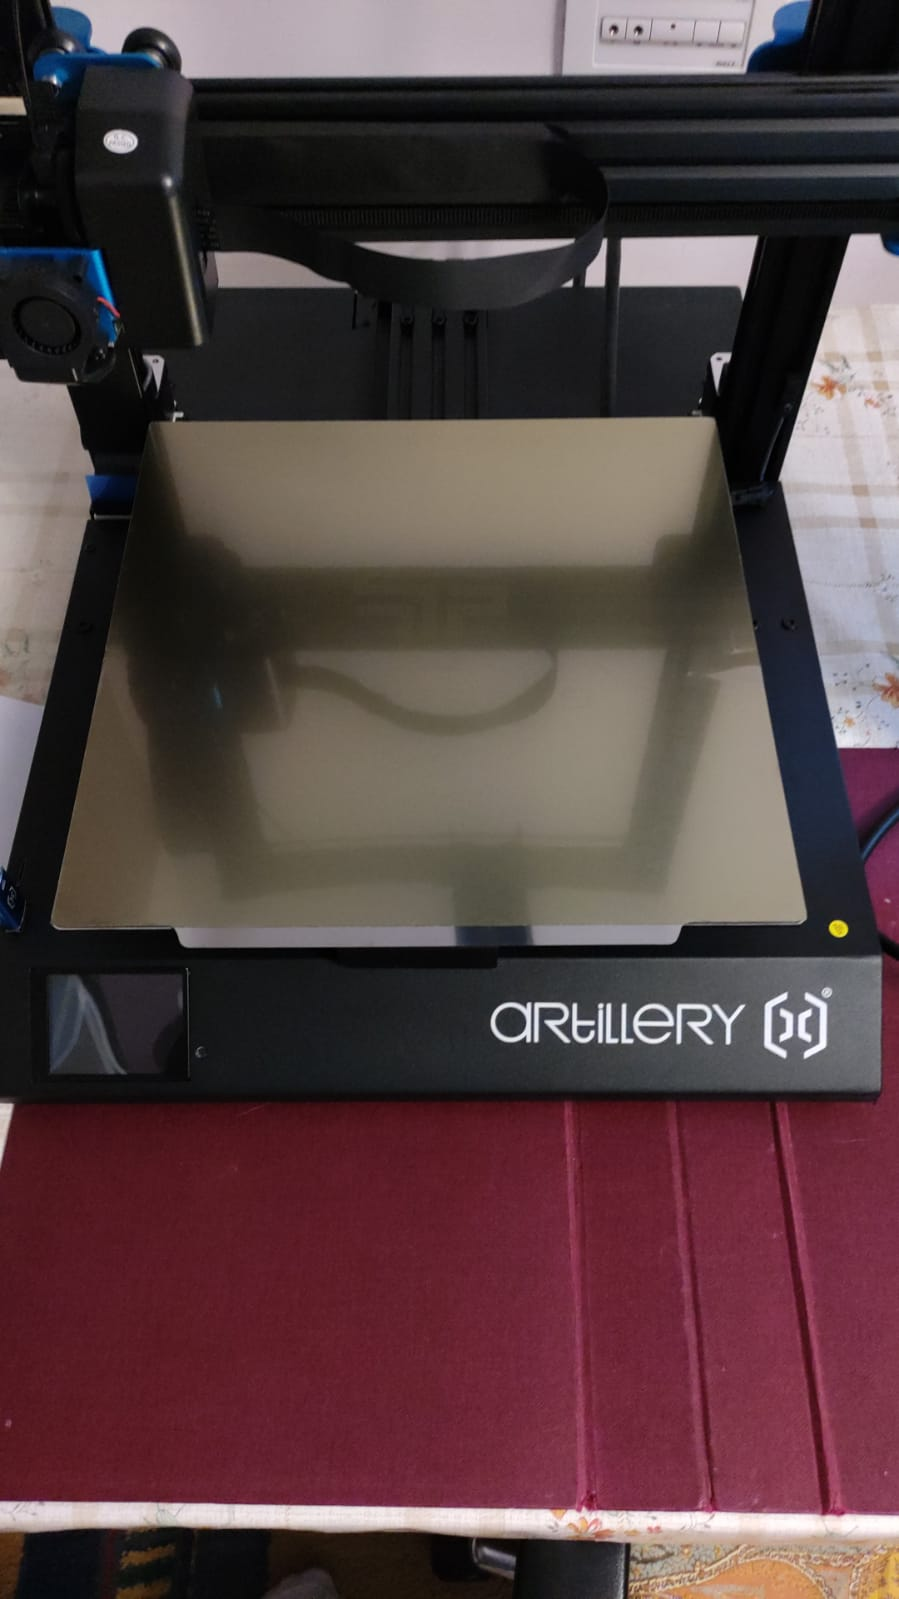}
\centering
\caption[Artillery 3D printer]{Our Artillery 3D printer}
\label{fig:3dprinter}
\end{figure}

\begin{figure}[!h]
\includegraphics[trim={0 0 0 0 },clip, width=0.7\textwidth]{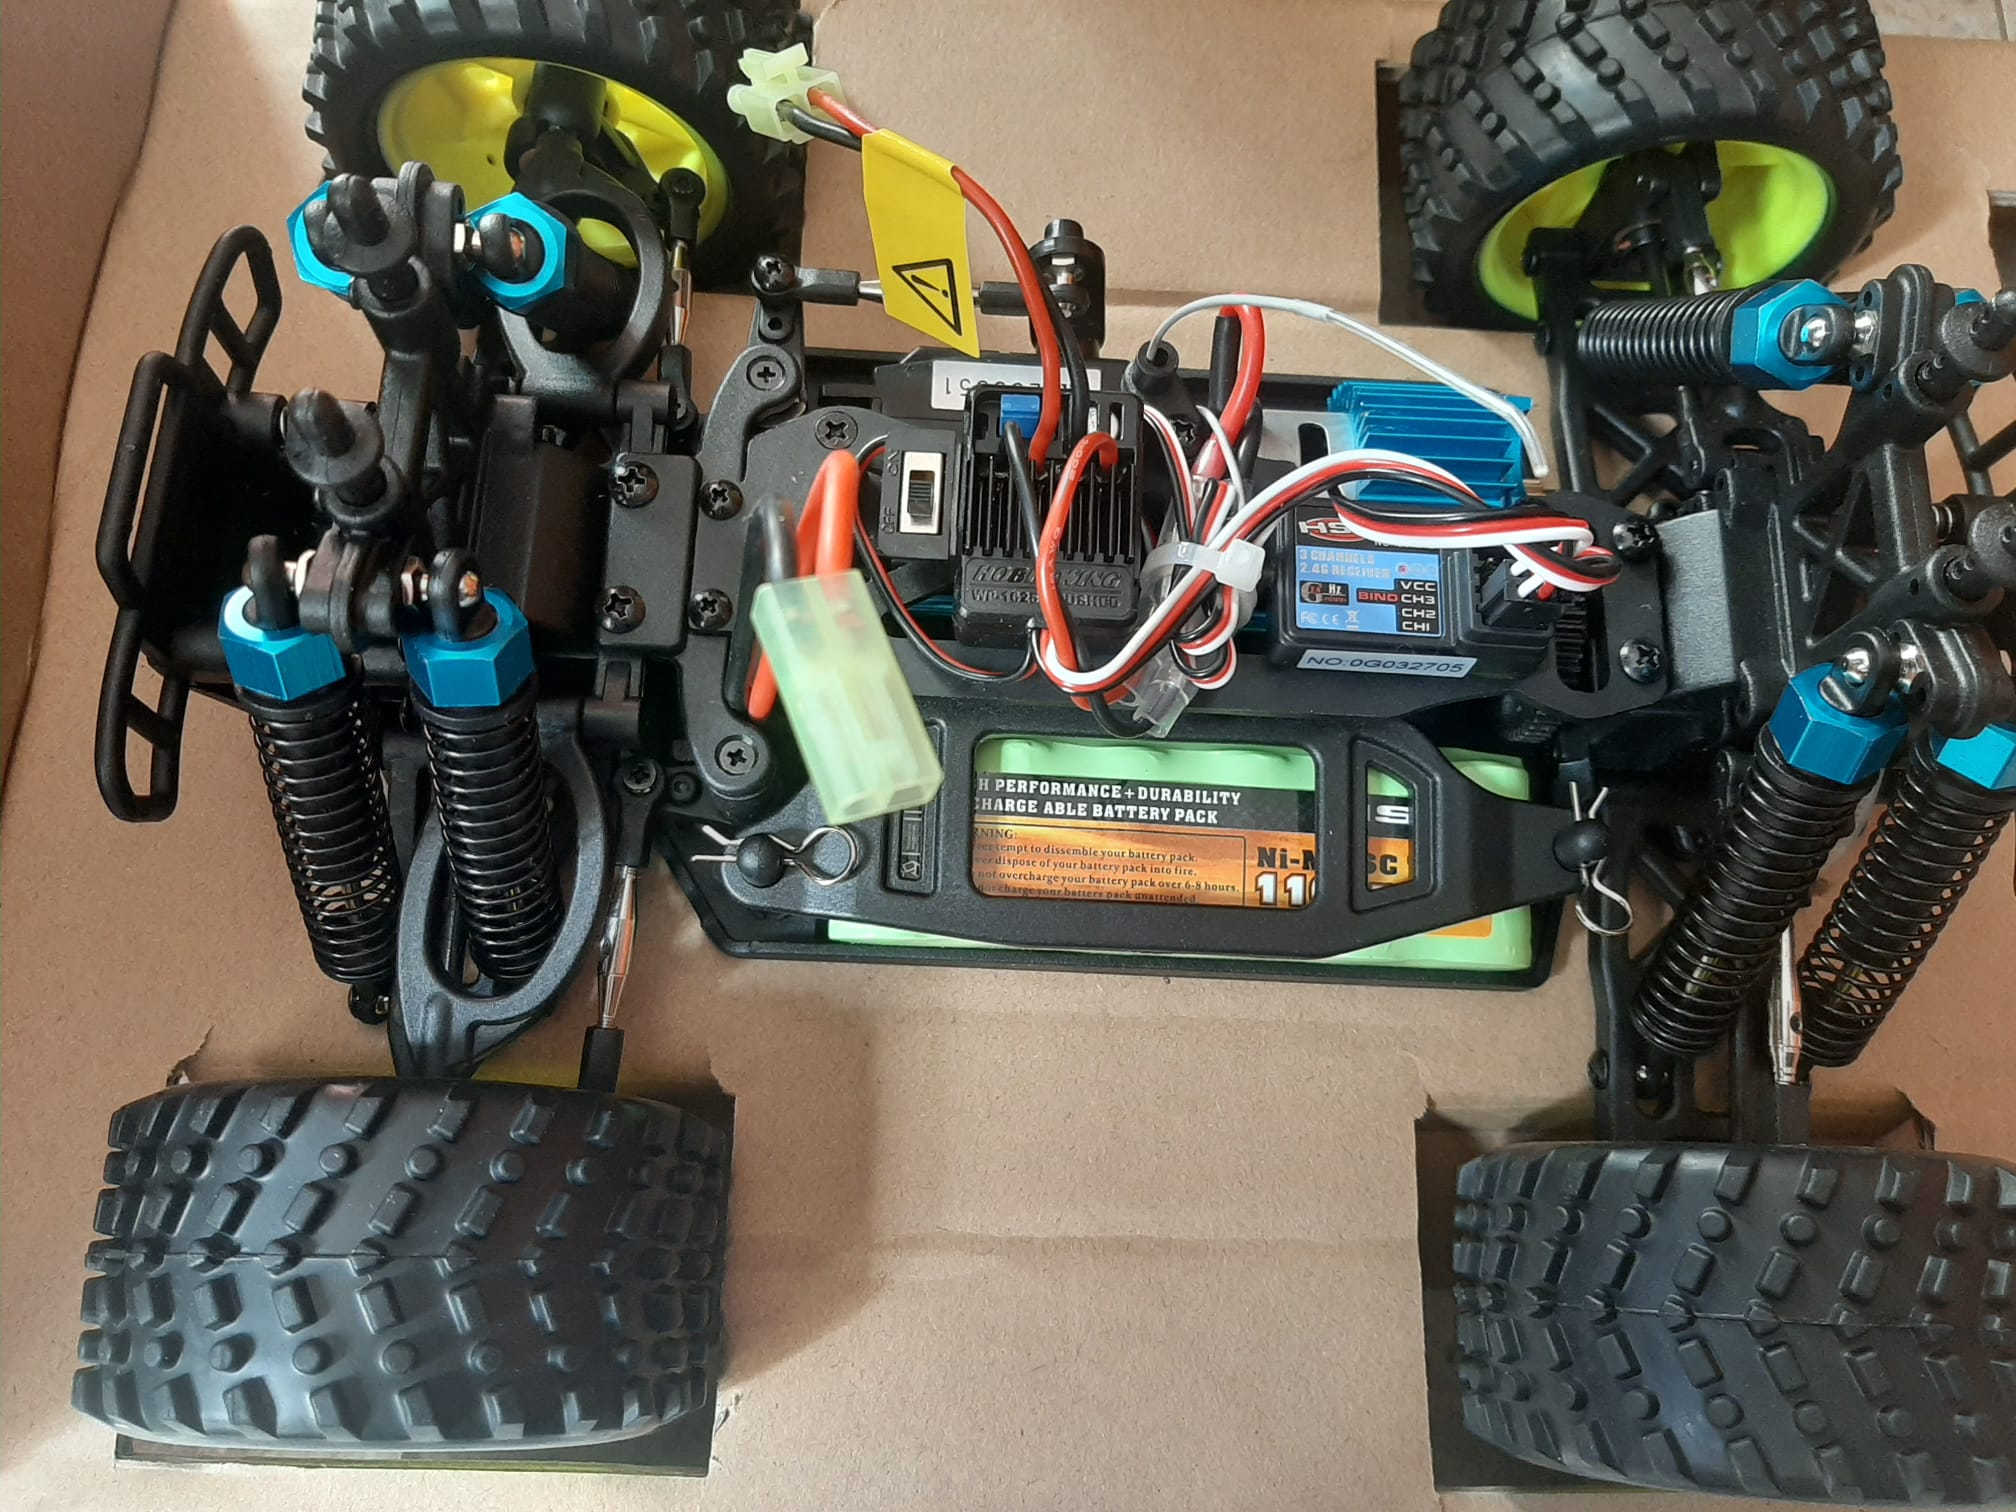}
\centering
\caption[Original DonkeyCar]{Original DonkeyCar}
\label{fig:donkey-car}
\end{figure}

%\begin{figure}[!h]
%\includegraphics[trim={0 0 0 0 },clip, width=\textwidth]{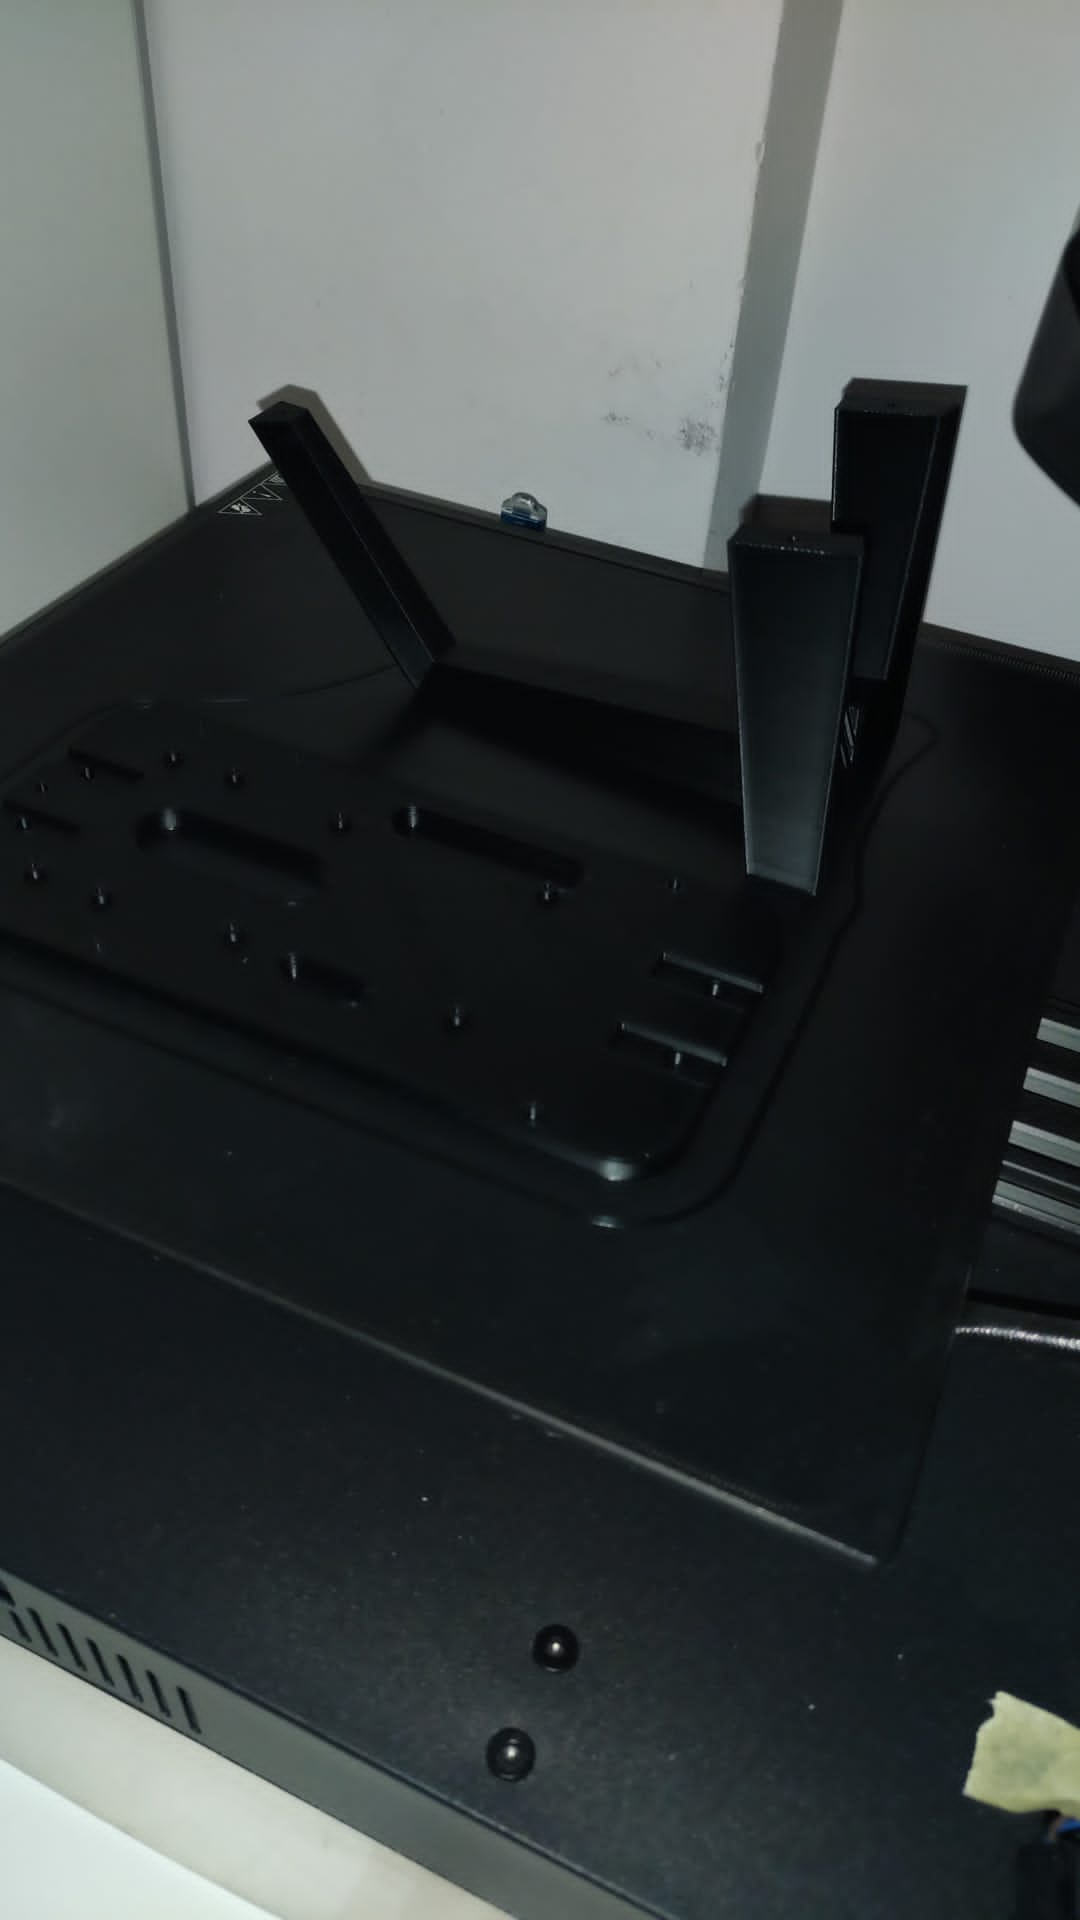}
%\centering
%\caption[JetRover: 3D printed parts]{JetRover: 3D printed parts}
%\label{fig:jet3dparts}
%\end{figure}

\begin{figure}[!h]
\includegraphics[trim={0 0 0 0 },clip, width=0.75\textwidth]{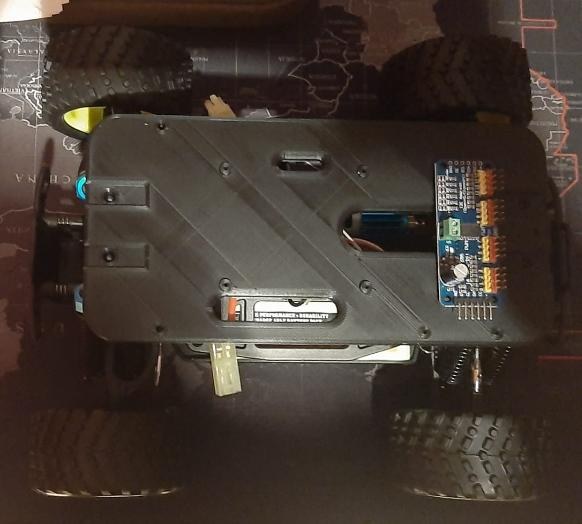}
\centering
\caption[JetRover 3D printed pieces]{JetRover 3D printed pieces}
\label{fig:jetrover-3d}
\end{figure}

\begin{figure}[!h]
\includegraphics[trim={0 0 0 0 },clip, width=0.85\textwidth]{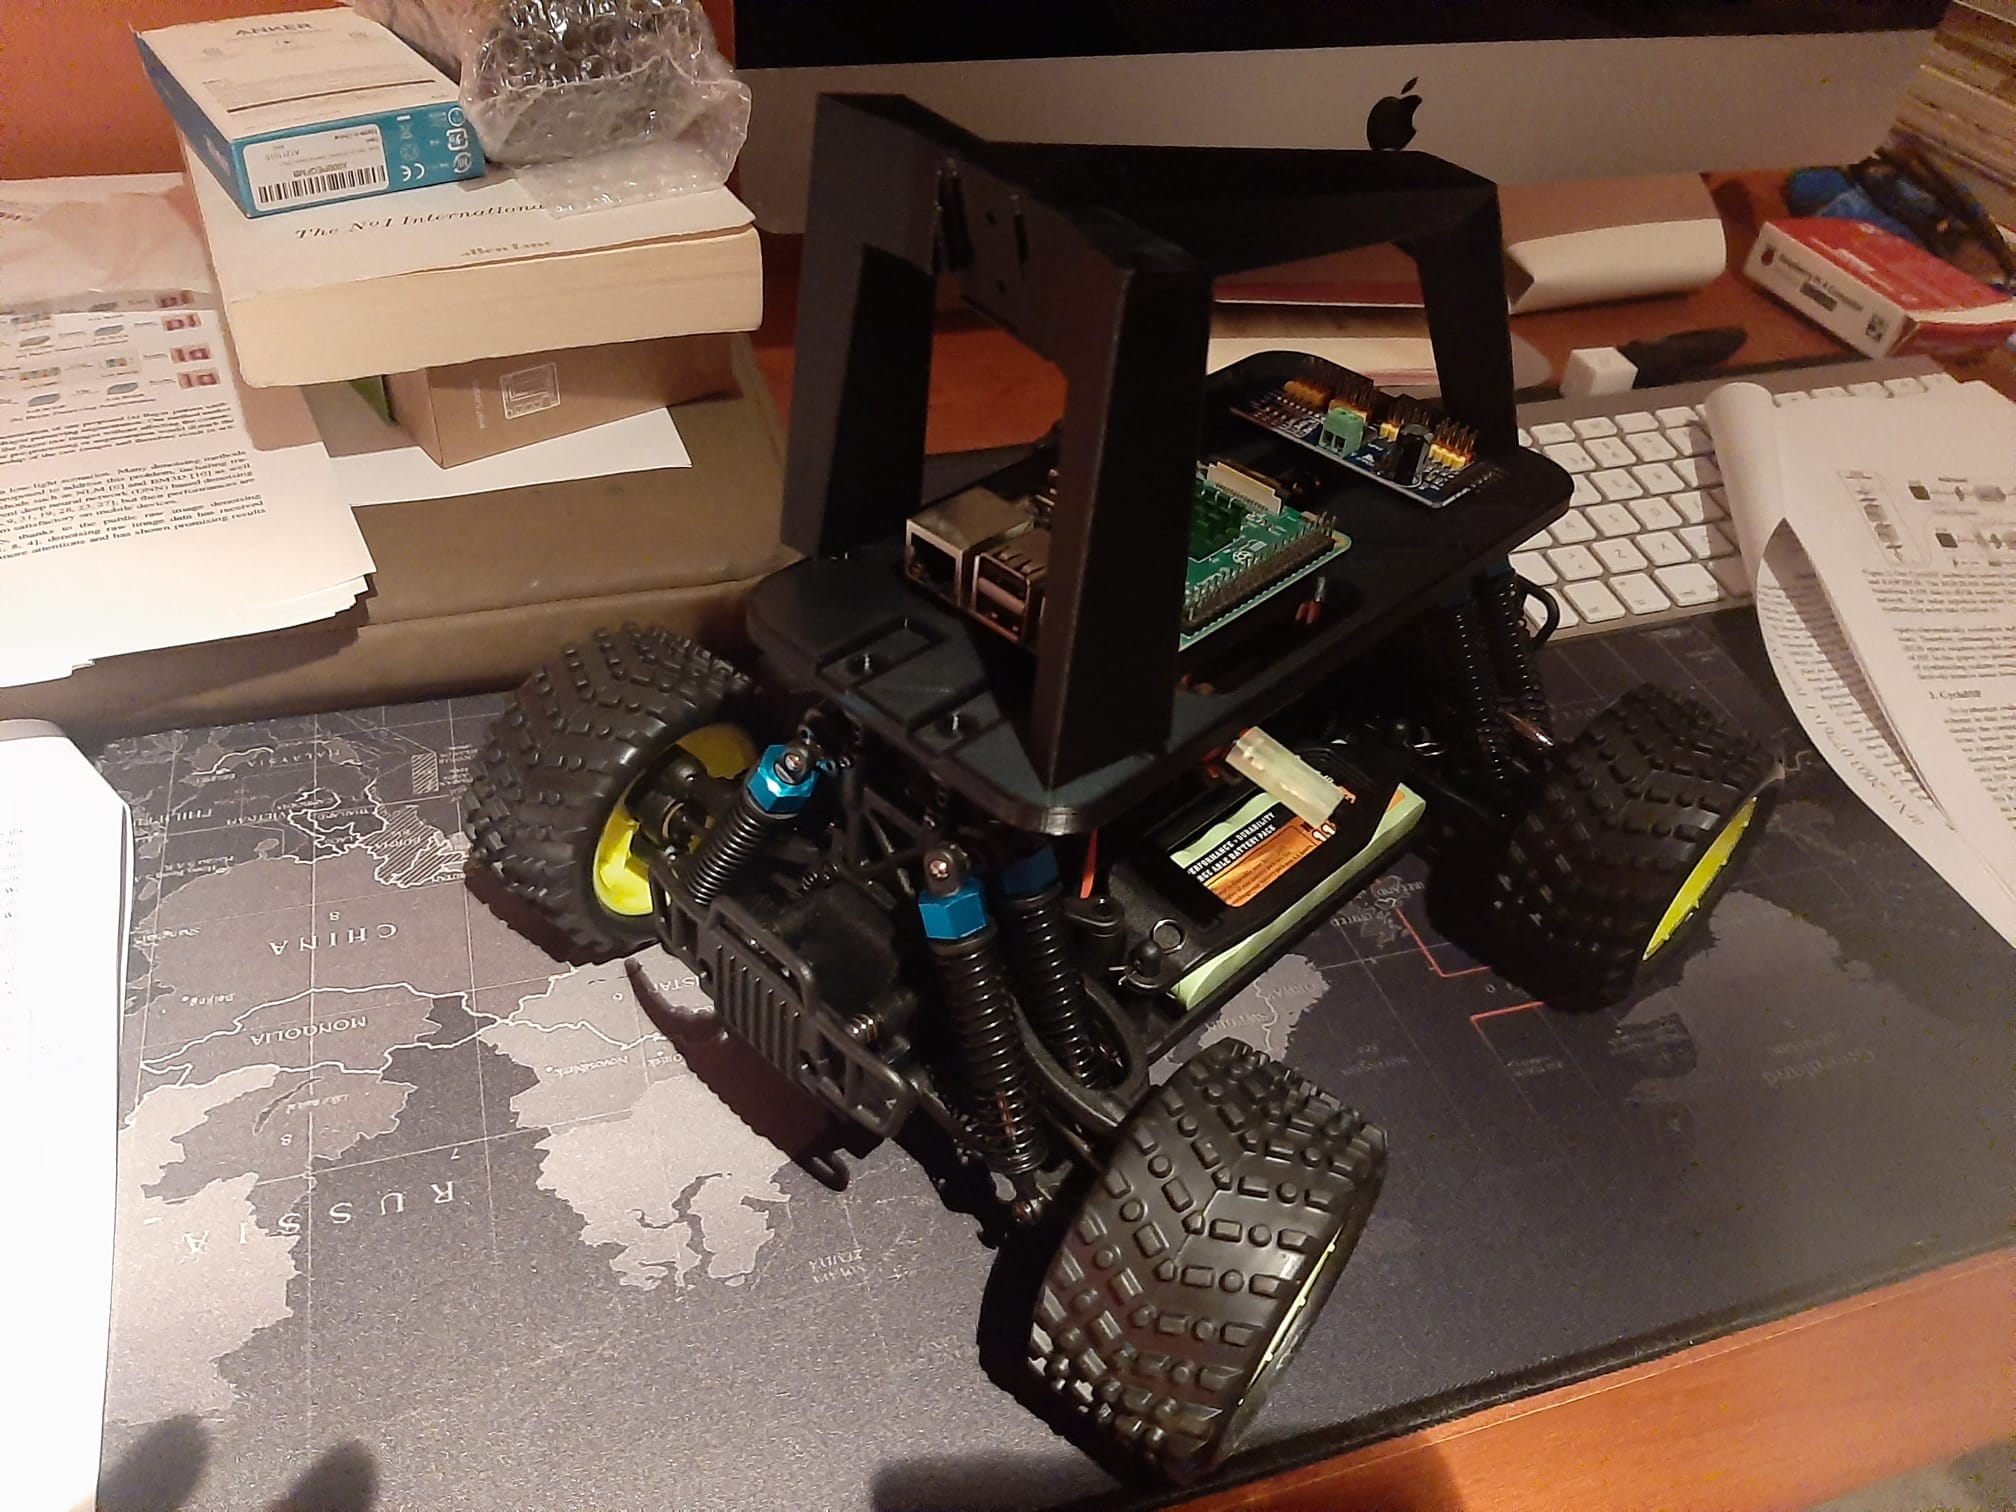}
\centering
\caption[JetRover photo 2]{JetRover with Raspberry Pi}
\label{fig:jetrover2}
\end{figure}

\begin{figure}[!h]
\includegraphics[trim={0 12cm 0 0 },clip, width=\textwidth]{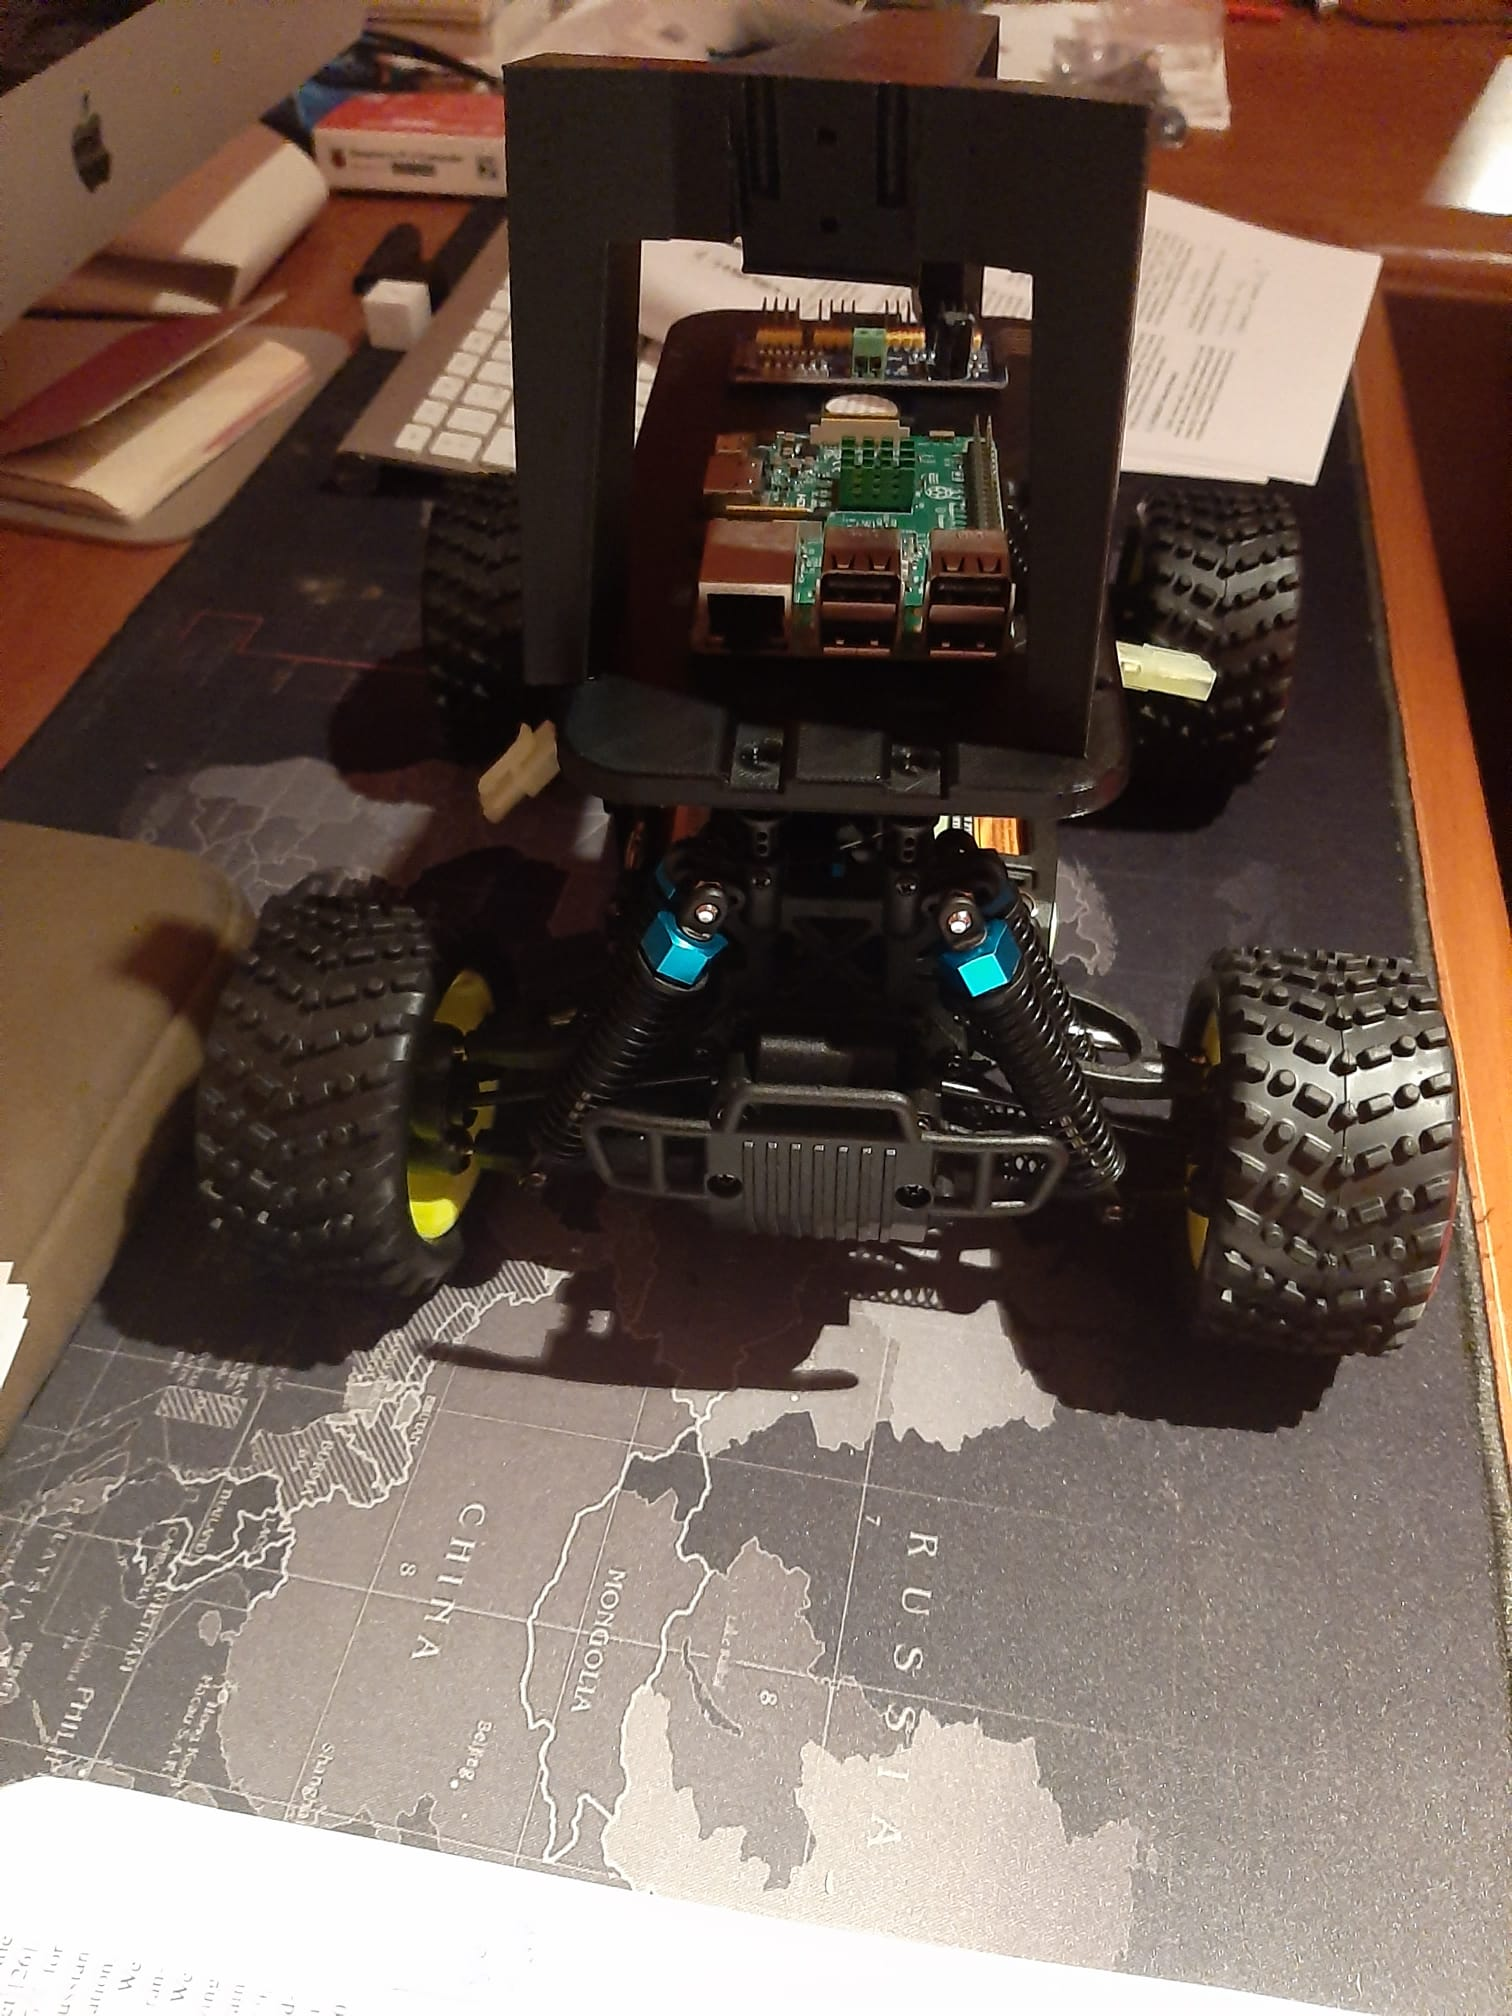}
\centering
\caption[JetRover photo 1]{JetRover}
\label{fig:jetrover1}
\end{figure}

\clearpage

Inspired by DonkeyCar \footnote{\url{https://www.donkeycar.com/}}, an opensource DIY self driving platform for small scale cars (RC CAR + Raspberry Pi + Python). Donkey is a Self Driving Car Platform for hobby remote control cars. Donkey Car consists of: (i) a high level self driving library written in Python. It was developed to enable fast experimentation and easy contribution. (ii) an Open Source Hardware design that makes it easy for you to build your own car (iii) a community of enthusiasts, developers and data scientists.
\\
We first bought a RC Car HSP 94186 standard chassis (Figure \ref{fig:donkey-car}), and using our own 3D printer (see Figure \ref{fig:3dprinter}), and the public available 3D models ($.stl$ files) \footnote{\url{https://www.thingiverse.com/thing:4309677}} we print the required parts in 8hrs. We reuse most hardware from the JetBot robot, thus, the cost of this robot is +150\$.
Figures \ref{fig:jetrover-3d}, \ref{fig:jetrover2}, and \ref{fig:jetrover1} show the building process of the robot following the official tutorials.

After installing the required Donkey packages \footnote{\url{https://docs.robocarstore.com/guide/robot_sbc/setup_jetson_nano/}}, we use the same technologies as we employed on JetBot (only motor drivers and API needed to be changed).
